# Supplementary material for: Enhancing the Accuracy of XPS Calculations: Exploring Hybrid Basis Set Schemes for CVS-EOMIP-CCSD Calculations
Source: arXiv:2411.03492 ancillary file (2024-11-05)
Supplement: Supplementary file 1 [file si.pdf]

# Supporting Information: Enhancing the Accuracy of XPS Calculations: Exploring Hybrid Basis Set Schemes for CVS-EOMIP-CCSD Calculations

Alexis A. A. Delgado, Devin A. Matthews*

*Department of Chemistry, Southern Methodist University,*

*3215 Daniel Ave, Dallas, Texas 75275-0314, USA*

E-mail: damatthews@smu.edu

# Role of Diffuse Functions: Additional Data

Fig. S1 shows the individual and statistical errors for hybrid mixed augmented/non-augmented basis sets [aug-$n/m$, $m/m$, $m$], with and without the frozen core approximation applied. In each case, additional diffuse functions are only included on the active atom.

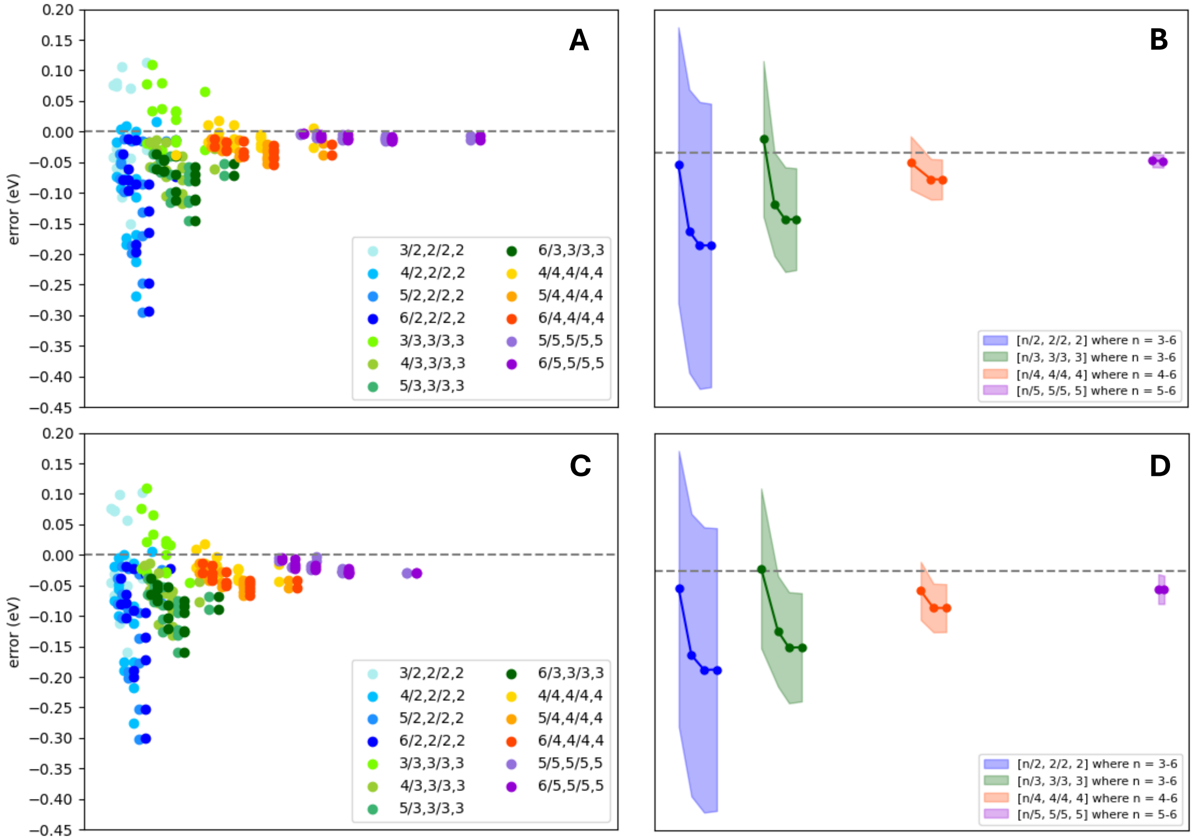


Figure S1: Errors in vertical IEs with respect to the estimated CBS limit for CVS-EOMIP-CCSD with hybrid mixed augmented basis sets combined with non augmented standard basis sets (hybrid mixed aug/non-aug basis sets) with and without FC applied. **A,C**: scatter plots of individual data showing the relationship between error and basis set size (number of b.f.s per atom). **B,D**: points represent average error for each basis set combination, and the shaded region indicates the 95% confidence interval over the test set. **A,B**: augmented hybrid basis sets on active atoms, and non-augmented standard basis sets on other atoms (hybrid mixed aug/non-aug basis sets). **C,D**: augmented hybrid basis sets on active atoms with frozen core approximation and non-augmented standard basis sets (with no tight core functions) applied to other atoms (frozen core hybrid mixed aug/non-aug basis sets).
